# Supplementary material for: Joint Local Relational Augmentation and Global Nash Equilibrium for Federated Learning with Non-IID Data
Source: arXiv:2308.11646 source file (2023-08-17)
Supplement: Supplementary file 1 [file appendix.tex]

\subsection{Convergence Analysis}
